# Supplementary material for: A Practical Mixed Precision Algorithm for Post-Training Quantization
Source: arXiv:2302.05397 source file (2023-02-10)
Supplement: Supplementary file 1 [file 08_appendix.tex]

\subsection{Quantizer Group}
